# Supplementary material for: An uncertainty-aware framework for data-efficient multi-view animal pose estimation
Source: arXiv:2510.09903 source file (2025-10-10)

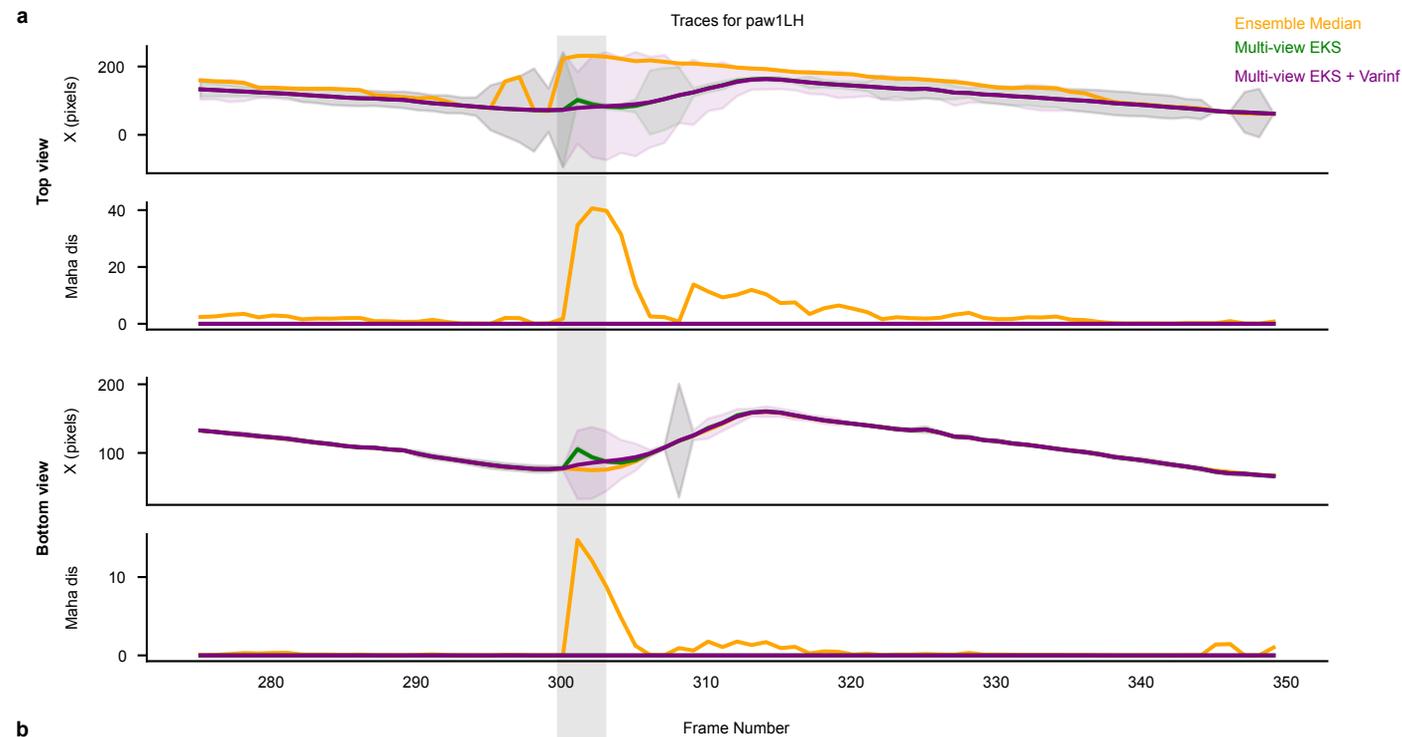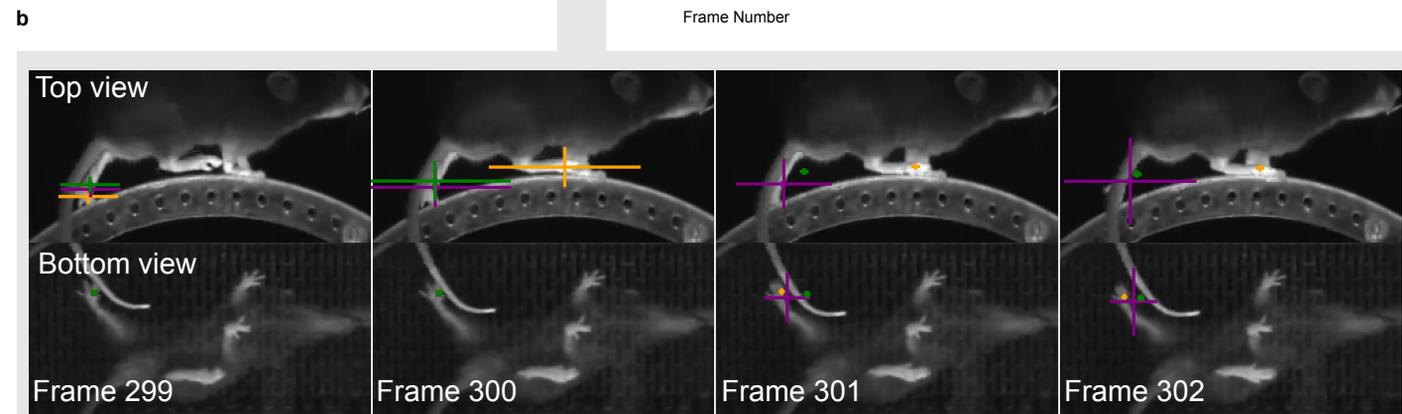

Supplement: Supplementary file 1 [file traces_paw1LH.pdf]
